# Supplementary material for: Two-dimensional Bloch electrons in perpendicular magnetic fields: an exact calculation of the Hofstadter butterfly spectrum
Source: arXiv:1303.2020 source file (2013-03-08)
Supplement: Supplementary file 1 [file SupplementaryInfoPRL.pdf]

# Two-dimensional Bloch electrons in perpendicular magnetic fields: an exact calculation of the Hofstadter butterfly spectrum (Supplementary Information)


S. Janecek,[1,2,3,4] M. Aichinger,[3] and E. R. Hernández[1,2]

[1] *Instituto de Ciencia de Materiales de Madrid (ICMM–CSIC), Campus de Cantoblanco, 28047 Madrid, Spain*
[2] *Institut de Ciencia de Materials de Barcelona (ICMAB–CSIC), Campus de Bellaterra, 08193 Barcelona, Spain*
[3] *Johann Radon Institute for Computational and Applied Mathematics (RICAM), Austrian Academy of Sciences, Altenberger Strasse 69, A-4040 Linz, Austria*
[4] *MathConsult GmbH, Altenberger Strasse 69, A-4040 Linz, Austria*



(Dated: March 8, 2013)


## MAGNETIC TRANSLATION GROUP AND GENERALIZED BLOCH THEOREM

We consider the single-particle Schrödinger equation,

$$H\psi(\mathbf{r}) \equiv \left[\frac{1}{2m}\Pi^2 + V(\mathbf{r})\right]\psi(\mathbf{r}) = E\psi(\mathbf{r}), \tag{1}$$

where $H$ is the Hamiltonian, $\psi(\mathbf{r})$ is an eigenstate with energy $E$, $\mathbf{\Pi} = \mathbf{p} + e\mathbf{A}(\mathbf{r})$ is the dynamical momentum operator and $\mathbf{A}(\mathbf{r})$ is the vector potential corresponding to the magnetic field, $\mathbf{B} = \nabla \times \mathbf{A}$. We take the field to be uniform and oriented along the $z$-direction, $\mathbf{B} = B\,\mathbf{e}_z$. The electrons are restricted to the two-dimensional (2D) $xy$-plane, and the external potential $V(\mathbf{r})$ is periodic on a Bravais lattice defined by vectors

$$\mathbf{R_n} = j\mathbf{a} + k\mathbf{b}, \;\; \mathbf{n} = (j,k) \in \mathbb{Z}^2. \tag{2}$$

To find symmetry operations that commute with the Hamiltonian $H$, we start by defining the conjugate momentum operator, $\bar{\mathbf{\Pi}} = \mathbf{p} + e\bar{\mathbf{A}}(\mathbf{r})$, where $\bar{\mathbf{A}}(\mathbf{r})$ is the conjugate vector potential. For linearly gauged vector potentials, i.e., $\mathbf{A}(\mathbf{r}) = \mathcal{J}\mathbf{r}$ with a constant Jacobian $\mathcal{J}$, the conjugate potential is $\bar{\mathbf{A}}(\mathbf{r}) \equiv \mathcal{J}^T\mathbf{r}$. A more general definition can be found in the review article [3]. With the conjugate momentum operator, we define a family of *magnetic translation operators* [1–3],

$$T_A(\mathbf{R_n}) \equiv \exp\left(-\mathrm{i}\pi jk\,\alpha\right)\,\exp\left(\frac{\mathrm{i}}{\hbar}\bar{\mathbf{\Pi}}\cdot\mathbf{R_n}\right), \tag{3}$$

where $\alpha = \frac{1}{2\pi}\frac{e}{\hbar}\left(\mathbf{a}\times\mathbf{b}\right)B$ is the magnetic flux through one unit cell in units of the flux quantum $\phi_0 = h/e$, and $\mathbf{R_n}$ is given by Eq. (2). These operators can be interpreted as translations with an additional gauge transform to reverse the effect of the translation on the vector potential. It is fairly straight-forward to show that they commute with the Hamiltonian Eq. (1), and have the property

$$T_A(\mathbf{R}_2)T_A(\mathbf{R}_1) = \exp\left[\mathrm{i}2\pi j_1k_2\,\alpha\right]T_A(\mathbf{R}_1+\mathbf{R}_2), \tag{4}$$

where $\mathbf{R}_1 = j_1\mathbf{a} + k_1\mathbf{b}$ and $\mathbf{R}_2 = j_2\mathbf{a} + k_2\mathbf{b}$ [3]. The operators $T_A(\mathbf{R_n})$ thus do not form a proper group, but a "group up to a phase factor". The situation is considerably simplified in the case of a *rational field*, $\alpha = p/q$, where $p$ and $q$ are relatively prime integers. In this case, the phase factor in Eq. (4) is a $q$-th root of unity for any lattice translation, and the product of the cyclic group of $q$-th roots of unity and the set of operators $T_A(\mathbf{R_n})$ form a group, the so-called *magnetic translation group* $\mathcal{G}$ [3]. The limit of irrational flux has also been studied by several authors, see, e.g. Ref. [4].

We now choose a subset of the the lattice $\mathbf{R}_n$, Eq. (2), such that its (larger) primitive cell encloses a number $p$ of flux quanta, e.g.,

$$\mathbf{S_n} = j\mathbf{a} + k(q\mathbf{b}), \;\; \mathbf{n} = (j,k) \in \mathbb{Z}^2. \tag{5}$$

The phase factor in Eq. (4) is then equal to one on this *magnetic lattice*, and the operators $T_A(\mathbf{S_n})$ form a normal abelian subgroup of $\mathcal{G}$, from which its irreducible standard representations can be calculated [3]. The zero-field Bloch situation is now almost restored: the unitary operators $T_A(\mathbf{S_n})$ fulfill $T_A(\mathbf{S}_2)T_A(\mathbf{S}_1) = T_A(\mathbf{S}_1+\mathbf{S}_2)$. Their eigenvalues thus must be of the form

$$T_A(\mathbf{S_n})\phi(\mathbf{r}) = e^{\mathrm{i}\boldsymbol{\theta}\mathbf{S_n}}\phi(\mathbf{r}) \tag{6}$$

with a constant vector $\boldsymbol{\theta}$, and we use the Bloch ansatz $\phi(\mathbf{r}) \equiv e^{\mathrm{i}\boldsymbol{\theta}\mathbf{r}}u^{\boldsymbol{\theta}}(\mathbf{r})$ for their eigenfunctions. For the subsequent calculations, we use an orthorhombic lattice formed by vectors $\mathbf{a} = a\,\mathbf{e}_x, \mathbf{b} = b\,\mathbf{e}_y$ and Landau gauge, $\mathbf{A}(\mathbf{r}) = Bx\mathbf{e_y}$. Substituting the definition of the magnetic translation operators, Eq. (3), into Eq. (6) yields the *generalized Bloch condition* [3] for the functions $u^{\boldsymbol{\theta}}(\mathbf{r})$,

$$u^{\boldsymbol{\theta}}(\mathbf{r}+\mathbf{S}) = \exp\left[-\mathrm{i}\frac{e}{\hbar}BS_xy\right]u^{\boldsymbol{\theta}}(\mathbf{r}), \tag{7}$$

where the *magnetic crystal momentum* $\boldsymbol{\theta}$ can be restricted to the *magnetic Brillouin zone* $-\pi/a \leq \theta_x \leq +\pi/a$, $-\pi/(qb) \leq \theta_y \leq +\pi/(qb)$. It is thus sufficient to calculate $u^{\boldsymbol{\theta}}(\mathbf{r})$ on a finite domain, i.e., the primitive cell of the magnetic lattice. As $H$ commutes with the operators $T_A(\mathbf{S_n})$, we can seek its eigenstates among the family of functions $\phi(\mathbf{r}) = e^{\mathrm{i}\boldsymbol{\theta}\mathbf{r}}u^{\boldsymbol{\theta}}(\mathbf{r})$. Substituting $\phi(\mathbf{r})$

into Eq. (1) yields a differential equation for the unknown functions $u^{\boldsymbol{\theta}}(\mathbf{r})$,

$$H(\boldsymbol{\theta})u_j^{\boldsymbol{\theta}}(\mathbf{r}) \equiv \big[T(\boldsymbol{\theta}) + V(\mathbf{r})\big]u_j^{\boldsymbol{\theta}}(\mathbf{r}) = E_j(\boldsymbol{\theta})u_j^{\boldsymbol{\theta}}(\mathbf{r}), \quad (8)$$

where the kinetic energy operator $T(\boldsymbol{\theta}) = \frac{1}{2m}(\Pi_x^2 + \Pi_y^2)$ in the Landau gauge chosen above has

$$\Pi_x^2 = -\hbar^2\left(\partial_x + \mathrm{i}\theta_x\right)^2; \Pi_y^2 = -\hbar^2\left(\partial_y + \mathrm{i}\theta_y + \frac{\mathrm{i}e}{\hbar}Bx\right)^2. \quad (9)$$

The symmetry property (7) can be exploited in a very elegant way [5]: the periodicity of the functions $u^{\boldsymbol{\theta}}(\mathbf{r})$ in the $y$-direction allows to expand them as a Fourier series,

$$u^{\boldsymbol{\theta}}(x,y) = \sum_{n=-\infty}^{\infty} \tilde{u}^{\boldsymbol{\theta}}(x,n)\ \exp\left(\mathrm{i}2\pi\frac{n}{bq}y\right). \quad (10)$$

The Bloch condition (7) for the Fourier coefficients $\tilde{u}^{\boldsymbol{\theta}}$ then reads

$$\tilde{u}^{\boldsymbol{\theta}}(x+a,n) = \tilde{u}^{\boldsymbol{\theta}}(x,n+p), \quad (11)$$

which reveals that every $p$-th coefficient function $\tilde{u}^{\boldsymbol{\theta}}(x,n)$ is identical up to a shift of $a$ in the $x$-direction. For large $x$, the term proportional to $B^2x^2$ in $\Pi_y^2$ dominates over the periodic potential; the functions $\tilde{u}^{\boldsymbol{\theta}}(x,n)$ thus decrease exponentially in this limit and only need to be considered on a finite interval.

## NUMERICAL SOLUTION OF THE SCHRÖDINGER EQUATION

To calculate the $n$ lowest eigensolutions of the eigenvalue problem (8), we have used the diffusion method: the evolution operator in imaginary time, $\mathcal{T}(\varepsilon) = \exp(-\varepsilon H)$, is repeatedly applied to a set of trial states $u_j(\mathbf{r}), j = 1\ldots n$, which are orthogonalized after every step. To efficiently calculate the action of the operator exponential, we have used a recently developed high-order factorization scheme to split $\exp[-\varepsilon(T+V)]$ into terms that contain the exponentials of $T$ and $V$ alone [6]. The exponential of $T = \frac{1}{2m}(\Pi_x^2 + \Pi_y^2)$ can be split further using an exact factorization scheme based on the harmonic-oscillator-like commutator relations of $\Pi_x^2$ and $\Pi_y^2$ [7]. Using these two methods together, the resulting factorization of the evolution operator is

$$\mathcal{T}\left[-\varepsilon H(\boldsymbol{\theta})\right] = \sum_{\ell=1}^{n} c_\ell \left[e^{-\frac{\varepsilon}{2\ell}V}\, e^{-\frac{\varepsilon}{2m\ell}C_e(\xi)\Pi_y^2}\right. \\ \left. e^{-\frac{\varepsilon}{2m\ell}C_c(\xi)\Pi_x^2} e^{-\frac{\varepsilon}{2m\ell}C_e(\xi)\Pi_y^2}\, e^{-\frac{\varepsilon}{2\ell}V}\right]^\ell + \mathcal{O}(\varepsilon^{2n+1}), \quad (12)$$

where the coefficients $c_\ell$, $C_e(\xi)$ and $C_c(\xi)$, with $\xi = \varepsilon\hbar eB/m$, are known analytically [6, 7]. We represent the wave functions $u_j^{\boldsymbol{\theta}}(\mathbf{r})$ and the potential $V(\mathbf{r})$ by their values on an equidistantly spaced real-space grid. In Landau gauge, with the operators $\Pi_x^2$ and $\Pi_y^2$ defined as in Eq. (9), the product of operators in Eq. (12) is applied to a function $u^{\boldsymbol{\theta}}(\mathbf{r})$ by performing the following steps:

1. The operator $V$ is diagonal in real space, $e^{-\frac{\varepsilon}{2\ell}V(\mathbf{r})}u^{\boldsymbol{\theta}}(\mathbf{r})$ is thus a simple point-wise multiplication on the real-space grid.
2. Calculate $\tilde{u}^{\boldsymbol{\theta}}(x,n)$ by a Fast Fourier Transform (FFT) of $u^{\boldsymbol{\theta}}(x,y)$ with respect to the $y$-component.
3. In $(x,n)$-space, $e^{-\frac{\varepsilon}{2m\ell}C_e(\xi)\Pi_y^2}\ \tilde{u}^{\boldsymbol{\theta}}(x,n)$ is again a point-wise multiplication, see Eq. (9).
4. Now regard $\tilde{u}^{\boldsymbol{\theta}}(x,n)$ as a set of $p$ one-dimensional functions $g_s^{\boldsymbol{\theta}}(x), s = 1\ldots p$, in the sense of Eq. (11). Fourier-transforming these functions yields $p$ functions $\tilde{g}_s^{\boldsymbol{\theta}}(k_x)$.
5. Again, $e^{-\frac{\varepsilon}{2m\ell}C_c(\xi)\Pi_x^2}\tilde{g}_s^{\boldsymbol{\theta}}(k_x)$ is a simple point-wise multiplication.
6. The remaining factors in the product can be applied by carrying out the above steps in reverse order.

## LOW-FIELD HOFSTADTER APPROXIMATION

For the low-field approximation to the magnetic spectrum we start with a TB model for the zero-field band structure of the square lattice,

$$\begin{aligned} E(\mathbf{k}) =& \gamma_{nn}\left(e^{ik_xa} + e^{+ik_ya} + \text{c.c.}\right) + \\ &+\gamma_{2nn}\left(e^{ik_xa}e^{ik_ya} + e^{ik_xa}e^{-ik_ya} + \text{c.c.}\right) + \\ &+\gamma_{3nn}\left(e^{2ik_xa} + e^{2ik_ya} + \text{c.c.}\right), \end{aligned} \quad (13)$$

where "c.c." means the complex conjugate of the previous terms. Here, $\gamma_{nn}, \gamma_{2nn}$ and $\gamma_{3nn}$ are the 1st, 2nd and 3rd nearest neighbor hopping integrals, which are used as fitting parameters, adjusted so as to reproduce the lowest three zero-field bands of the numerical calculation [shown in Fig. (1c)]. The fitting procedure was carried out over a regular grid of $\mathbf{k}$-points spanning the first Brillouin zone shown in Fig. (1b). It was found that the 1st neighbor hopping integral was sufficient to reproduce the lowest band, this case thus corresponding to Hofstadter's original model. For the remaining two bands also 2nd and 3rd nearest neighbor hoppings were needed. The fitted bands [shown in Fig. (1c) as dashed lines] reproduce the zero-field bands very well. We have then performed the Peierls substitution [8, 9] $\mathbf{k} \to (\mathbf{p} + e\mathbf{A})/\hbar$ in Eq. (13), where $\mathbf{p}$ is the momentum operator, using the Landau gauge $\mathbf{A}(\mathbf{r}) = Bx\mathbf{e}_y$ for the vector potential. This transforms $E(\mathbf{k})$ into an effective Hamiltonian, which can be diagonalized by standard LAPACK routines to obtain its dispersion relation, DOS and the Hall conductance in the mobility gaps $\sigma_{xy}^{\text{gap}}$ through Středa's formula.

[1] E. Brown, Phys Rev A-Gen Phys **133**, 1038 (1964).
[2] J. Zak, Phys Rev A-Gen Phys **134**, 1607 (1964).
[3] H. J. Fischbeck, Phys Status Solidi **38**, 11 (1970).
[4] G. Obermair and G. Wannier, *Phys. Status Solidi B* **76**, 217–222 (1976).
[5] W. Cai and G. A. Galli, *Phys. Rev. Lett.* **92**, 186402 (2004).
[6] S. A. Chin, S. Janecek and E. Krotscheck., *Chem. Phys. Lett.* **470**, 342–346 (2009).
[7] M. Aichinger, S. A. Chin and E. Krotscheck, *Comp. Phys. Comm.* **171**, 197–207 (2005).
[8] R. Peierls, *Z. Physik* **80**, 763 (1933).
[9] J. Luttinger, *Phys. Rev.* **84**, 814–817 (1951).
